# Supplementary material for: Lipid membrane domains control actin network viscoelasticity
Source: arXiv:2406.13218 ancillary file (2024-10-22)
Supplement: Supplementary file 1 [file Arnold_Takatori_Supplement_2024.pdf]

# SUPPLEMENTAL MATERIAL:

## Lipid membrane domains control actin network viscoelasticity

Daniel P. Arnold and Sho C. Takatori\*

*Department of Chemical Engineering, University of California, Santa Barbara, Santa Barbara, CA 93106*

### I. VIDEO DESCRIPTIONS

**Video S1:** Comparison of actin relaxation on single- and two-phase lipid membranes. (*Left*) Actin filaments (cyan) are adsorbed to a planar lipid membrane (not shown) consisting of a single liquid-disordered (Ld) phase, and allowed to relax over time. (*Right*) Actin filaments (magenta) are adsorbed to a two-phase lipid membrane containing dispersed liquid-ordered (Lo) droplets in a Ld continuous phase. Over time, the Lo domains coarsen, driving accelerated actin relaxation compared to the Ld-only membrane. The membrane and its Lo and Ld phases are not shown, but the Lo droplets occupy the voids in the actin network and can be seen in Video S2. Scale bars are 5  $\mu\text{m}$ .

**Video S2:** Actin and lipid domain relaxation. Fluorescence micrographs show: (*upper left*) a two-phase lipid bilayer with liquid-ordered (Lo, green) domains in a liquid-disordered (Ld, black) continuous phase, (*upper right*) an actin network (magenta) adsorbed to the Ld phase, and (*lower center*) both actin and Lo domains overlaid. As time progresses, the actin network relaxes and yields, allowing Lo domains to grow and coarsen.

**Video S3:** Tracer actin filament fluctuation. Tracer actin filaments, truncated by gelsolin to a length of  $\approx 1 \mu\text{m}$ , are tracked over a period of  $\approx 20 \text{ s}$ . The short time-lapses are collected 0 min (left), 6 min (center), and 14 min (right) after cholesterol addition begins. Filament centers are tracked over the 20-second period and the variance plotted in Fig. 3C of the main text. Scale bar is 2.5  $\mu\text{m}$ .

### II. SUPPLEMENTAL NOTES

#### Note 1: Use of different samples for actin structure measurement and tracer filament tracking

For the experiments in which cholesterol is added into the membrane using methyl beta-cyclodextrin (m $\beta$ CD), we use one sample to measure the structure of bulk actin and lipid domains, and another to measure tracer actin fluctuations.

After using N-hydroxysuccinimide (NHS) chemistry to label G-actin with multiple Alexa Fluor dyes, we find that Alexa Fluor 555 provides a bright, and relatively bleach-resistant signal. Thus, in all of the experiments presented in the main text, we present actin labeled with NHS-Alexa Fluor 555. Moreover, 1,2-distearoyl-sn-glycero-3-phosphoethanolamine-N-[poly(ethylene glycol)2000-N'-carboxyfluorescein] DSPE-PEG2k-FITC is the only lipid-based dye we find to have sufficient affinity for the Lo phase to distinctly label the domains. Thus, with Lo and actin fluorescing at 488 nm and 555 nm, respectively, we try Alexa Fluor 647-labeled tracer actin filaments (Fig. S2A). While in our earliest experiment, we did not use gelsolin to truncate the tracer filaments (making them relatively long), Fig. S2A still clearly shows that the Alexa Fluor 647 is relatively dim, making tracer filaments difficult to track. Moreover, after several tracking time-lapses, the Alexa Fluor 647 bleaches considerably. Thus by 15 minutes, many of the smaller filaments become almost invisible.

To maximize tracer filament intensity, and thus maximize tracking accuracy, we instead label tracer filaments with Alexa Fluor 555 for our production-quality tracking experiments (Fig. S2B). The gelsolin-truncated filaments labeled with Alexa Fluor 555 in Fig. S2B are much more distinct than their Alexa Fluor 647-labeled counterparts in Fig. S2A and do not bleach nearly as much over the course of the experiment. After 14 minutes, they remain clearly differentiated from the background. However, to keep the tracer signal relatively clean and free of cross-talk, we are forced to use Alexa Fluor 405 to label the bulk actin in. Alexa Fluor 405 has poor a signal-to-noise ratio (Fig. S2B, left), which will sacrifice sensitivity in the fast Fourier transforms needed to measure the mean actin wavelength  $\xi$ .

Thus in the main text, we maintain separate samples for tracer tracking and actin/Lo structural analysis. Due to the variability in cholesterol insertion rate between samples, the exact time values in Fig. 4C of the main text should not be directly compared to those in Fig. 4A-B. However, the qualitative trends are consistent.

---

\* stakatori@ucsb.edu

### III. SUPPLEMENTAL FIGURES

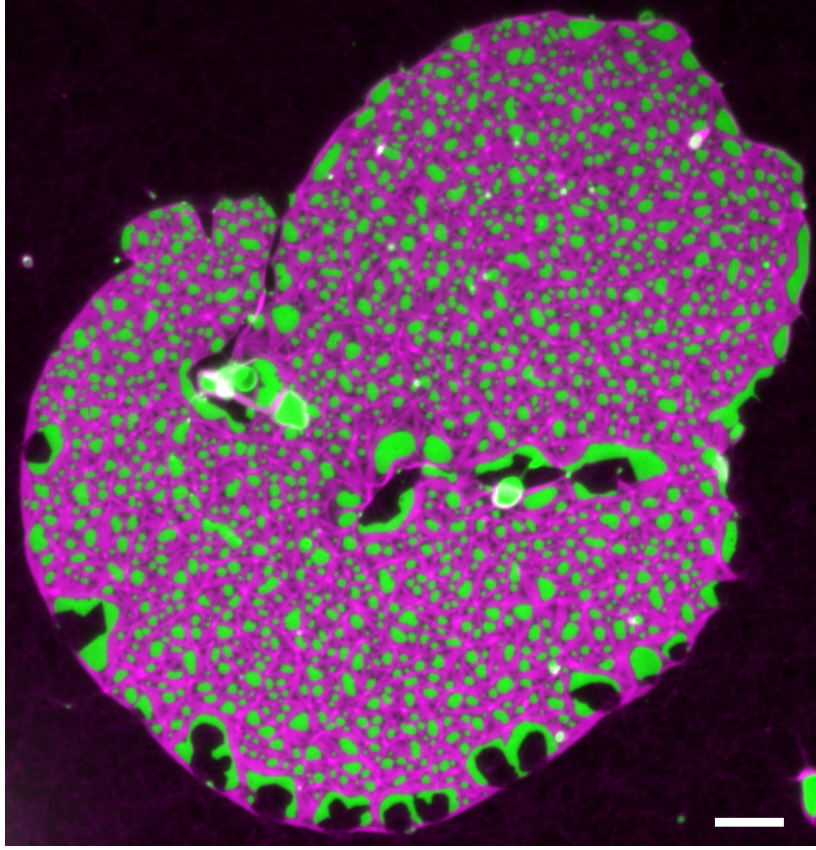

FIG. S1. Fluorescence micrograph of a two-phase lipid membrane with adsorbed actin, cropped such that all edges of the membrane are visible. Planar lipid membranes containing dispersed liquid-ordered (Lo, green) domains in a liquid disordered (Ld, not shown) continuous phase are created by rupturing a giant unilamellar vesicle (GUV) on a treated glass coverslip. Once the GUVs splatter, their membranes spread into an oblong “splatter” on the coverslip surface, which is approximately round, and may be over 100  $\mu\text{m}$  in size. We then adsorb filamentous actin (magenta) to the membrane, which only wets the Ld area of the membrane, avoiding the Lo domains. Thus, in this image the magenta regions roughly correspond to the Ld phase of the membrane, while the black areas on the perimeter are outside the membrane “splatter” area and have no color. Scale bar is 10  $\mu\text{m}$ .

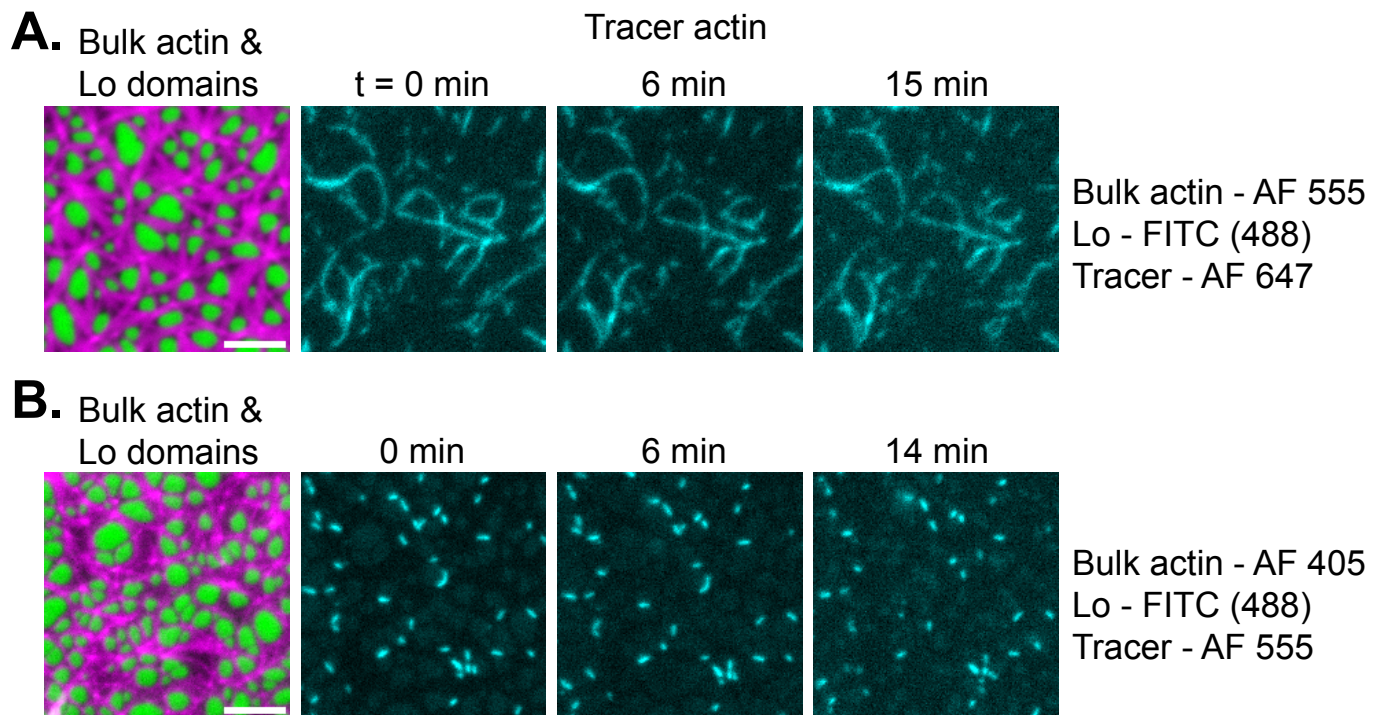

FIG. S2. Tracer filament fluctuation and actin/domain structure are measured on different samples for cholesterol insertion experiments. (A) In experiments studying Lo domain and bulk actin structure, Alexa Fluor 555-labeled bulk actin and FITC-labeled Lo domains are considered (left). In such samples, Alexa Fluor 647 is the best candidate for labeling tracer actin filaments, but it is dim and bleaches over the course of the experiment (right). Tracers here are not truncated with gelsolin, and are thus relatively long. (B) In experiments studying tracer fluctuations, we use Alexa Fluor 555-labeled actin to maximize accuracy (right). To avoid cross-talk and tracer signal contamination, we must use Alexa Fluor 405-labeled bulk actin with FITC-labeled Lo domains (left). The Alexa Fluor 405-labeled actin has a poor signal-to-noise ratio, making it less optimal for structural analysis. All scale bars are 5  $\mu\text{m}$ .
